# Supplementary material for: APRICOT: Active Preference Learning and Constraint-Aware Task Planning with LLMs
Source: arXiv:2410.19656 source file (2024-10-25)
Supplement: Supplementary file 1 [file perception_detail.tex]

\subsection{Perception}
We will use the static camera to identify the objects already in the fridge and to determine the occupied space for geometric feasibility purposes. Because we assume that we have a set of object labels already, the goal of the perception module is to (1) identify each object in the fridge with its name and bounding box and (2) extract its semantic locations so that the LLM-based task planner can easily understand the information. 

For the (1) goal, directly using an open-vocabulary object detector~\cite{liu2023grounding}, which can simultaneously output the label and bounding box, is challenging due to the wide range of grocery item names. The object detector is sensitive to hyperparameters and struggles to balance between false negatives (not detecting the objects that are in the fridge) and false positives (detecting objects that are in the fridge). To overcome this, we decompose this step into two parts (Fig.~\ref{fig:e2e_failure_cases}): first, we only focus on extracting the bounding boxes of objects in the fridge without needing to label them with specific names; second, we find the best label for those extracted bounding boxes. 

\textbf{Detect Object Bounding Box: } We use GroundingDINO ~\cite{liu2023grounding} with a fixed text prompt "grocery item" to put bounding boxes around all of the objects in the fridge. Empirically, we observe that sometimes GroundingDINO draws boxes around larger objects (e.g. fridge) or draws multiple boxes around the same object. Thus, we use a threshold to filter out bounding boxes that are too large and Non-Maximum Suppression to filter out overlapping bounding boxes. 

\textbf{Label Object Bounding Box: } For each bounding box detected, we crop the image into $I_i$ encode it using CLIP~\cite{radford2021learning} to get CLIP embeddings $\phi_{CLIP} (I_i)$. For the dataset of potential object labels $L_i$, we also encode them with CLIP~\cite{radford2021learning} to get CLIP embeddings $\phi_{CLIP}(L_i)$. We find the best label for a bounding box cropped image $I_i$ by finding the best object name $L$ that maximizes the cosine similarity between the CLIP embeddings:
\begin{equation*}
    \argmax_{L} \frac{\phi_{CLIP} (I_i) \phi_{CLIP} (L)}{|| \phi_{CLIP} (I_i) || || \phi_{CLIP} (L) ||}
\end{equation*}

\textbf{Extract Semantic Locations: } Because the task planner is using an LLM, a semantic location (e.g. `top shelf`) is more informative compared to numerical values from a bounding box. With the ArUco tags on a shelf, we can detect the shelf's bounding box. For each detected object, its semantic location is determined based on where its bounding box is with respect to the shelf's bounding box.
